# Supplementary material for: Proximity-induced topological phases in bilayer graphene
Source: arXiv:1802.04396 source file (2018-02-12)
Supplement: Supplementary file 1 [file Supplementary_Materials.pdf]

# Proximity-induced topological phases in bilayer graphene

## Supplementary Materials

## I. TIGHT-BINDING MODEL

In this section we introduce the tight-binding formalism used to study the BLG-TMD heterostructure, and discuss the validity of its numerical intralayer coupling parameters.

First of all, due to the incommensurability of the graphene and TMD lattices, one defines supercells that contain multiples of each lattice cell to reduce the overall remnant strains. We focus on two different heterostructures that are expected to capture the relevant features of the structure. They are 3×3 TMD cells with 4×4 graphene units in each layer, and 4×4 TMD with 5×5 graphene. Our results show to be qualitatively similar for these two different heterostructure sizes at low energy and it does not change the main conclusions discussed in the main text.

The tight-binding Hamiltonian that couples nearest neighbor ($\langle ij \rangle$) $p_z$-orbitals in graphene and third-nearest-neighbor metal atoms in TMD, each with three relevant $d$-orbitals ($d_{z^2}$, $d_{x^2-y^2}$ and $d_{xy}$), can be written as[1,2]

$$\mathcal{H}_{\rm T} = \sum_{i,\nu,\sigma} \epsilon_\nu \boldsymbol{\alpha}^\dagger_{i\nu\sigma}\boldsymbol{\alpha}_{i\nu\sigma} + \sum_{\langle ij\rangle,\nu,\mu,\sigma} t_{m_{ij},\nu\mu}\boldsymbol{\alpha}^\dagger_{i\nu\sigma}\boldsymbol{\alpha}_{j\mu\sigma} + h.c.,$$
$$\mathcal{H}_{\rm Gl} = \sum_{i,l,\sigma} \epsilon_{il\sigma}\boldsymbol{c}^\dagger_{il\sigma}\boldsymbol{c}_{il\sigma} - t_g \sum_{\langle ij\rangle,l\sigma} \boldsymbol{c}^\dagger_{il\sigma}\boldsymbol{c}_{jl\sigma} + h.c., \tag{1}$$

where $\alpha$ and $\boldsymbol{c}$ are operators for TMD and graphene atoms, respectively, and $l$ describes the graphene layer number, $l = 1, 2$. The indices $\mu$ and $\nu$ indicate the orbital degrees of freedom. The first term in $\mathcal{H}_T$ considers the on-site energy of atom $i$ and orbital $\nu$. The second term describes hopping between metal atom orbitals to their neighbors. The spin orbit coupling (SOC) in TMD originates mostly from the atomic contribution,[1] as seen in Eq. 25 and Table IV in Ref. 1.

For concreteness, we use two different characteristic TMD substrates, namely $WS_2$ and $MoS_2$. The material parameters are adopted from Liu *et al.*,[1] while in graphene we take a hopping parameter equal to $t_g$ = 3.033 eV.[2] The interlayer coupling between graphene $p_z$ and the metal atom $d$-orbitals is

$$\mathcal{H}_\perp = \sum_{\langle ij\rangle,\sigma} t^\gamma_{i,j}\boldsymbol{c}^\dagger_{i1\sigma}\boldsymbol{\alpha}_{j\gamma\sigma} + h.c., \tag{2}$$

where the interlayer coupling $t^\gamma_{i,j}$ to layer 1 (adjacent to the TMD) is represented by a tunneling amplitude

$$t^\gamma_{i,j} = t_\gamma \exp\left[-|\boldsymbol{r}_{m,j} - \boldsymbol{r}_{g,i}|/\eta\right], \tag{3}$$

where $\eta = 5a_g$ is a normalization constant, and $|\boldsymbol{r}_{m,i} - \boldsymbol{r}_{g,j}|$ is the distance between atoms in the TMD and graphene layers. The TMD-graphene layer separation is taken as 3.66 Å, as reported from density functional calculations,[3] and also close to recently reported experimental results.[4] We neglect the coupling between the TMD and the distant graphene layer, as the large intervening van der Waals gaps would strongly suppress such direct coupling.

The tunneling is parameterized via Slater-Koster orbital couplings between the graphene $p_z$ orbitals and $d$-orbitals of the TMD monolayer using[5]

$$\begin{aligned} t^{d_{z^2}} &= \langle p_z|H|d_{z^2}\rangle \\ &= \sqrt{3}n_z(n_x^2+n_y^2)V_{pd\pi} - \frac{1}{2}n_z(n_x^2+n_y^2-2n_z^2)V_{pd\sigma} \\ t^{d_{x^2-y^2}} &= \langle p_z|H|d_{x^2-y^2}\rangle \\ &= \left(\frac{\sqrt{3}}{2}V_{pd\sigma} - V_{pd\pi}\right) n_z(n_x^2-n_y^2) \\ t^{d_{xy}} &= \langle p_z|H|d_{xy}\rangle \\ &= n_x n_y n_z(\sqrt{3}V_{pd\sigma} - 2V_{pd\pi}), \end{aligned} \tag{4}$$

where $n_i$ are directional cosines. $V_{pd\pi}$ and $V_{pd\sigma}$ couple orbitals through $\sigma$ and $\pi$ bonds. The numerical values of these two parameters are estimated as −0.46 eV and 0.11 eV, respectively. These values are consistent with density functional calculations that have studied TMD-graphene layers,[6–8] and could easily be underestimated here.

The BLG is assumed to have Bernal stacking, typically favored over other stacking types. There are four coupling amplitudes between atoms in these two layers, the direct coupling parameter ($t_\perp = 0.3$eV) between on-registry A and B atoms being the largest.[9] For simplicity, we keep only the direct coupling since it effectively describes the low-energy regime.

The $z$-inversion symmetry can be broken due to the existence of a substrate or by applying an electric field that sets both graphene layers at different voltage. This asymmetry generates also a Rashba SOC effect that mixes spin states and plays an important role in the heterostructure properties. This effect adds a Rashba term to the tight-binding Hamiltonian of the graphene layers of the form[10]

$$\mathcal{H}_R = \sum_{\langle ij\rangle l\sigma\sigma'} t_{Rl}\,\hat{z}\cdot(\mathbf{s}_{\sigma\sigma'}\times\mathbf{d}^\circ_{ij})c^\dagger_{il\sigma}c_{jl\sigma'}\,, \tag{5}$$

where $\mathbf{d}^\circ_{ij}$ is the unit vector that connects nearest neighbor atoms A and B in each layer $l$. Reports of a Rashba spin orbit coupling induced on graphene suggest

this interaction to be $t_{R1} = 0.67$ meV and $t_{R2} = 1.67$ meV. An electric field applied perpendicularly to the heterostructure is modeled using $\sum_{il\sigma} V_{\text{Gate}}(l)\, c^{\dagger}_{il\sigma} c_{il\sigma}$, where $V_{\text{Gate}}(l)$ is the energy shift in each graphene layer $l$ produced by the applied voltage. The applied voltage can be seen as an overall shift of both graphene layers with respect to the TMD, which shifts the BLG neutrality point closer/away from the valence band of the TMD. In addition, the field configuration may include an asymmetric or *opposite* relative voltage between the two graphene layers. The overall shift is important, as energy proximity to the valence band enhances SO effects. However, the relative opposite voltage may also push the system away from a topological phase, as discussed below and in the main text. Notice the effective model Hamiltonian parameters reported below have an implicit dependence on the overall voltage shift.

## II. FITTING TO THE EFFECTIVE HAMILTONIAN

The main text shows that the effective Hamiltonian fits well the tight-binding band structure results. Fig. 1 here shows the relative positions of the graphene-like states to the TMD bands as the gate voltage changes. It is important to note that the proposed effective Hamiltonian is capable of describing not only the band structure correctly, but it also fully captures the spin $\langle S_z \rangle$ and AB pseudospin $\langle \sigma_z \rangle$ texture of the tight-binding eigenstates. These characteristics are calculated as

$$\langle S_z \rangle = \frac{\hbar}{2} \langle \Psi_i | \sigma_0 \otimes s_z | \Psi_i \rangle, \quad \langle \sigma_z \rangle = \langle \Psi_i | \sigma_z \otimes s_0 | \Psi_i \rangle, \quad (6)$$

where $\sigma_i$ and $s_i$ are Pauli matrices acting on its corresponding pseudospin and spin spaces, respectively, as in the main text. Results of these values help constrain the fit to the tight-binding band structure, and are shown in Fig. 2. The numerical values of the effective parameters used in Fig. 1 are summarized in Table I (see Eq. 2 in main text for Hamiltonian details). Notice in Table I that $\Delta$ ($S$) and $\delta$ ($\lambda$) have equal magnitude and opposite sign. This is as a result of fixing the Dirac points at the Fermi level ($E_{\text{F}} = 0$) regardless of the applied effective gate voltage.

| | BLG-$WS_2$ | | | | BLG-$MoS_2$ | | | |
|---|---|---|---|---|---|---|---|---|
| | Fig. 1a | | Fig. 1b | | Fig. 5b | | Fig. 5a | |
| Parameter | Layer2 | Layer1 | Layer2 | Layer1 | Layer2 | Layer1 | Layer2 | Layer1 |
| $\Delta$ | 0.06 | −0.24 | −5.68 | 2.74 | 1.64 | −0.40 | −6.46 | 3.57 |
| $\delta$ | −0.06 | −10.05 | 5.68 | 10.9 | −1.64 | −13.67 | 6.46 | 15.12 |
| $S$ | 1.33 | −0.26 | 0.03 | −0.54 | 1.56 | −0.35 | −0.09 | −0.28 |
| $\lambda$ | −1.33 | −3.86 | −0.03 | −2.66 | −1.56 | −2.27 | 0.09 | −1.60 |
| $R$ | 0.11 | 1.1 | 0.11 | 1.1 | 0.11 | 1.1 | 0.11 | 1.1 |

TABLE I. Effective parameter couplings fitted to the tight-binding results corresponding to BLG-$WS_2$ and BLG-$MoS_2$ heterostructures. Parameters correspond to fittings shown in Fig. 1a and b as well as Fig. 5a and b. Layer 1 is the closest to the TMD layer. All values are in $m$eV.

Next, we discuss the Berry curvature structure of the (occupied) valence bands near the gap shown in Fig. 1.

### A. Berry Curvature

The proximity of the TMD to BLG leads to a fully gapped system where the Fermi level lies in the gap. Since the low energy physics of the carriers is dominated by the $K$ and $K'$ valleys, we need to determine the Berry curvature in their neighborhood. In a system with time-reversal symmetry (TRS), the Berry curvature $\Omega(k)$ satisfies $\Omega(k) = -\Omega(-k)$, so that we can limit the calculation to one valley, such that

$$\Omega_n(\boldsymbol{k}) = -\sum_{n' \neq n} \frac{2\text{Im}\langle \Psi_{n'\boldsymbol{k}} | v_x | \Psi_{n\boldsymbol{k}} \rangle \langle \Psi_{n\boldsymbol{k}} | v_y | \Psi_{n'\boldsymbol{k}} \rangle}{(\epsilon_n - \epsilon_{n'})^2}, \quad (7)$$

where $n$ is the band number, and $v_x(v_y)$ is the velocity operator along the $x(y)$ direction.[11] Figure 3 shows the Berry curvatures for the two low-energy (valence) bands, near the $K$ point, for the system shown in Fig. 1. We emphasize that the total Berry curvature over the Brillouin zone is zero, consistent with TRS.

As seen in Fig. 3, the bands that are nearly flat have strong Berry curvature features around each valley, a distinguishing signature of the band inversions seen in Fig. 1, or Fig. 1 and 2 in the main text. This figure shows

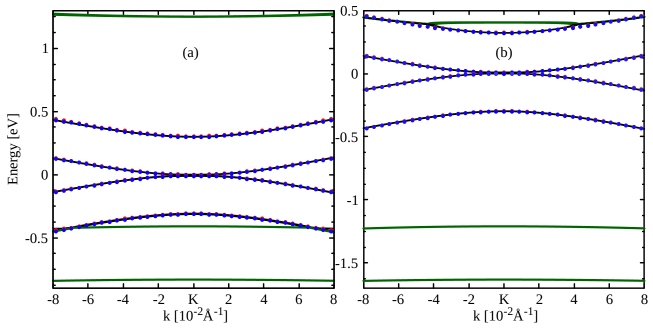


FIG. 1. Tight-binding band structure of BLG-TMD trilayer system near the $K$ valley, showing the relative position of the BLG bands with respect to the TMD conduction and valence bands (green flat lines). Application of a gate voltage shifts the neutrality point with respect to the TMD bandgap. (a) and (b) panels show results described in Fig. 2 in main text, with BLG parabolic bands shifted close to TMD valence band (a), or close to TMD conduction band (b). Red (blue) curves describe spin down (up) states. Circles represent the effective Hamiltonian fit, demonstrating excellent fit of the tight-binding band structure over several hundred meV range.

that the effective Hamiltonian also captures the subtle features of the tight-binding Berry curvature. To see the inversion of the bands more clearly, we tune a relative voltage difference in the system, which changes the flatness of the inverted bands around the $K$ points, as shown in Fig. 4. It is interesting to find that the topology of the bands, as indicated by their Berry curvature (not shown here), does not change over this range.

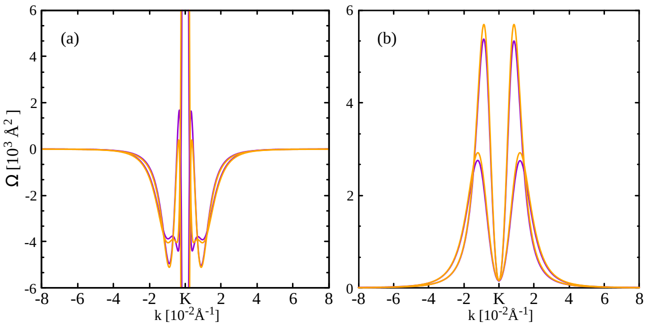


FIG. 3. (a) and (b) panels show Berry curvature of the topmost two valence bands in Fig. 1a and b, respectively. Both panels show that the effective Hamiltonian (orange lines) capture the curvature of the original tight banding model (violet lines)

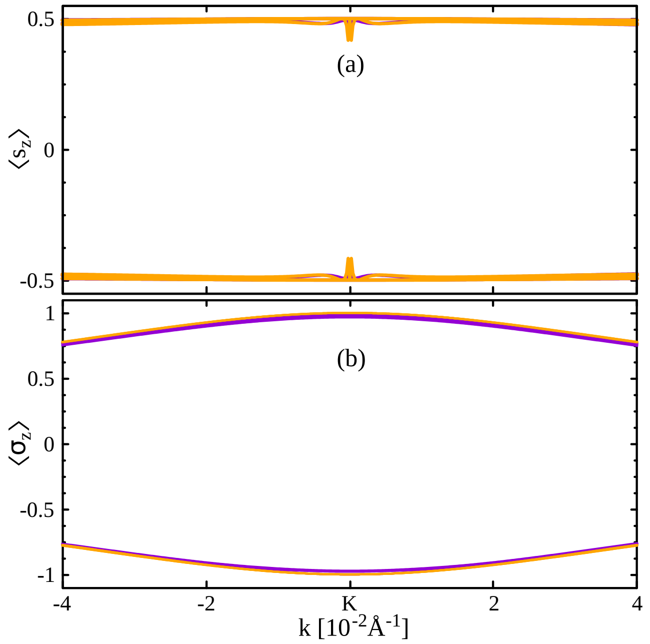


FIG. 2. (a) Spin and (b) staggered expectation values of the effective Hamiltonian fitted to the tight-binding model results for the system shown in Fig.1a. Notice fitting agrees well at the $K$ valley and diverges slowly away due mostly to hybridization with the valence bands of TMD that are very close here, as seen in Fig. 1a. Violet (orange) lines describe tight-binding (effective) Hamiltonian states, demonstrating full agreement of two models.

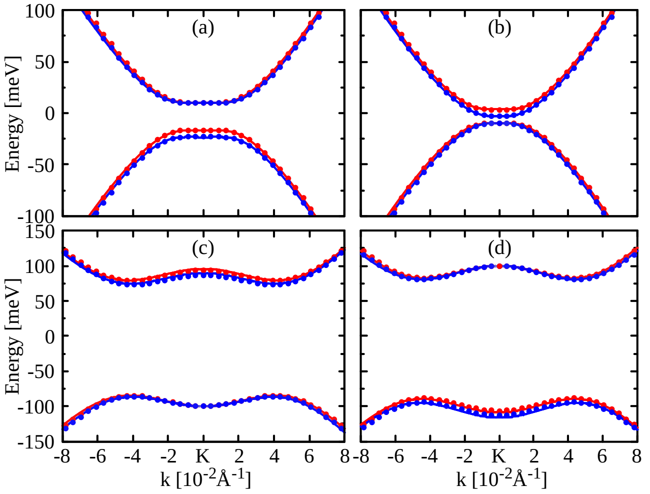


FIG. 4. Applying a gate voltage across the bilayer graphene sets the top and bottom layers at opposite voltage. (a) Panel describe a system at opposite voltage $V = 0.01$eV, (b) $V = -0.01$eV, (c) $V = 0.1$eV, and (d) $V = -0.1$eV. This results are for the BLG-$WS_2$ system shown in Fig. 1a. Clearly a larger $V$ enhances the full gap of the structure as in isolated BLG. Red (blue) color describes spin down (up) states. Circles represents effective Hamiltonian results.

## III. TMD SUBSTRATE AND INTERLAYER COUPLING PARAMETERS

In this section, we study the effect of changing the TMD substrate proximitizing bilayer graphene. Although the main text reported results when using $WS_2$ as a substrate, replacing $WS_2$ by $MoS_2$ produces similar qualitative features. For example, BLG-$WS_2$ shows a nearly 7 meV gap with a larger spin split due to stronger SOC. In contrast, BLG-$MoS_2$ exhibits a larger bulk gap, nearly 10 meV, with smaller spin splitting, as shown in Fig. 5a and 5b. Despite these numerical differences, band curvature features are similar, i.e., spin-split for either conduction or valence bands, whereas the other are nearly degenerate.

Panels 5c and 5d show also the effect of the interlayer couplings $V_{pd\pi}$ and $V_{pd\sigma}$ introduced in section I. As mentioned, they are estimated from density function calculations, with some uncertainty. To see the effect of these two parameters on the numerical results, we present results after multiplying their values by a factor of two. The resulting band structure of BLG-$MoS_2$ shows the same qualitative features with overall enhancements in gap and other effective parameters. We see in these panels that the gap and spin-splittings are generally larger by a factor of three–compare panel 5a and 5c, for example.

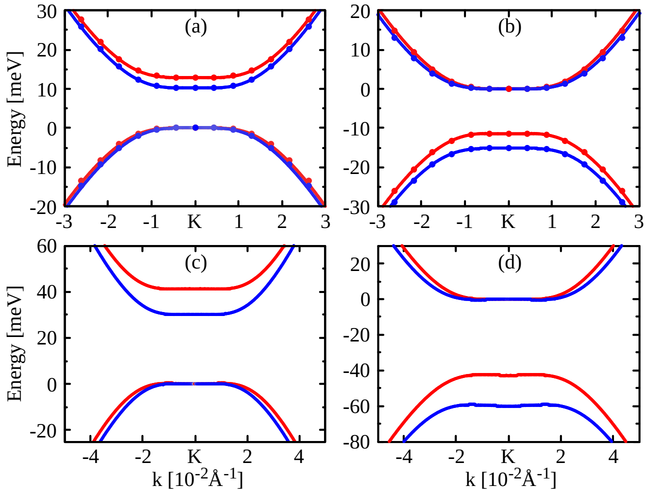


FIG. 5. Low energy band structure of BLG-$MoS_2$ multilayer system for two different interlayer coupling strengths of $V_{pd\pi}$ and $V_{pd\sigma}$, and for two different positions of the BLG neutrality point relative to the TMD bands. Red (blue) lines describe spin down (up) states obtained from tight-binding calculations. (a) and (b) uses the same parameters ($V_{pd\pi} = -0.46$ eV and $V_{pd\sigma} = 0.11$ eV) used in the main text. In (c) and (d) the couplings are doubled, with corresponding enhancement of bandgaps and spin splittings. In (a) and (c) the neutrality point of BLG is shifted close to the conduction band of TMD. In (b) and (d) the neutrality point is brought close to the valence band of TMD. Notice that (a) and (b) panels show the effective Hamiltonian correctly fit and describe the band structure of the tight-binding Hamiltonian using the fitted parameter introduced in Table I.

## IV. $Z_2$ INVARIANT

In this section, we briefly introduce the method used to calculate the $Z_2$ invariant based on a manifestly gauge-independent method.[12–14] It relies on examining the full non-Abelian adiabatic transport along time reversal paths in the rectangular Brillouin zone (BZ). This method does not require gauge fixing and uses a projection operator of the Bloch eigenstates for the occupied bands, $P_k = \sum_{i\in \text{occ. bands}} |u_i(\boldsymbol{k})\rangle \langle u_i(\boldsymbol{k})|$.

In a 2D BZ, unitary operations are generated by calculating the evolution along time reversal paths, $k_y = -\pi \to \pi$ at fixed $k_x = 0, \pi$:

$$U(k_i; k_f) = \prod_{n=1}^{N} P_k(k_n). \tag{8}$$

We take these paths and calculate evolution operators $U(k_i; k_f)$, with 2D-arguments $(k_{ix}, k_{iy}; k_{fx}, k_{fy})$ denoting paths

$$\begin{aligned}(0,-\pi;0,\pi) &= (0,-\pi) \to (0,\pi)\\ (\pi,-\pi;\pi,\pi) &= (\pi,-\pi) \to (\pi,\pi)\\ (0,0;0,\pi) &= (0,0) \to (0,\pi)\\ (\pi,0;\pi,\pi) &= (\pi,0) \to (\pi,\pi)\,.\end{aligned} \tag{9}$$

Using the same basis used to calculate $U(k_i, k_f)$, one constructs matrices with elements

$$\begin{aligned}U_{ij}^{(1)} &= \langle u_i(0,\pi)\, |U(0,0;0,\pi)|\, u_j(0,0)\rangle\\ U_{ij}^{(3)} &= \langle u_i(0,\pi)\, |U(0,-\pi;0,\pi)|\, u_j(0,\pi)\rangle\\ U_{ij}^{(2)} &= \langle u_i(\pi,\pi)\, |U(\pi,0;\pi,\pi)|\, u_j(\pi,0)\rangle\\ U_{ij}^{(4)} &= \langle u_i(\pi,\pi)\, |U(\pi,-\pi;\pi,\pi)|\, u_j(\pi,\pi)\rangle\ ,\end{aligned} \tag{10}$$

and calculate the following matrices at time reversed points

$$\begin{aligned}W_{ij}^{(1)} &= \langle u_i(0,0)\, |\mathcal{T}|\, u_j(0,0)\rangle\\ W_{ij}^{(3)} &= \langle u_i(0,-\pi)\, |\mathcal{T}|\, u_j(0,\pi)\rangle\\ W_{ij}^{(2)} &= \langle u_i(-\pi,0)\, |\mathcal{T}|\, u_j(\pi,0)\rangle\\ W_{ij}^{(4)} &= \langle u_i(-\pi,-\pi)\, |\mathcal{T}|\, u_j(\pi,\pi)\rangle\,,\end{aligned} \tag{11}$$

where $\mathcal{T} = i\sigma_y\mathcal{C}$ is the time reversal operator and $\mathcal{C}$ is the complex conjugation. $W^{(i)}$ is antisymmetric, and for a square matrix of size 4 has the form

$$W_{ij}^{(i)} = \begin{pmatrix} 0 & a & b & c\\ -a & 0 & d & e\\ -b & -d & 0 & f\\ -c & -e & -f & 0\end{pmatrix}. \tag{12}$$

The Pfaffian of $W^{(i)}$ is in general $\text{Pf}(W^{(i)}) = \sqrt{\det[\text{W}^{(i)}]}$, which for Eq. 12 yields $\text{Pf}(W^{(i)}) = af -$

$be + dc$. Thus, the $Z_2$ invariants are evaluated using

$$Z_2 = \pm 1 = \frac{\mathrm{Pf}(W^{(1)})\mathrm{Pf}(W^{(3)})}{\mathrm{Pf}(W^{(2)})\mathrm{Pf}(W^{(4)})} \frac{\det[\mathrm{U}^{(1)}]\det[\mathrm{U}^{(3)}]}{\sqrt{\det[\mathrm{U}^{(2)}]}\sqrt{\det[\mathrm{U}^{(4)}]}} . \quad (13)$$

Lastly, there is a canonical way to fix the ambiguity in the $Z_2$ sign in this equation, for systems with broken inversion symmetry.[12] This is done by monitoring the branch of the square root of $\sqrt{\det[\mathrm{U}^{(2)}]}$ as $k_x$ changes from 0 to $\pi$ ($\sqrt{\det[\mathrm{U}^{(4)}]}$). We count the number $n$ of crossings of the branch line (-∞,0] in the complex plane, and then correct $Z_2 \to Z_2 \times (-1)^n$.

Finally, we mention that this method is evaluated using a rectangular or square arbitrary real space lattice.[14] Thus, in bilayer graphene, the smallest supercell lattice to study $Z_2$ is rectangular and includes 4 atoms per unit cell per layer.

### A. Phase diagram

The main text studied a phase diagram of Rashba couplings where the BLG neutrality point is close to the valence bands of TMD, corresponding to Fig. 1a and left column of Table I. Here, we complete the analysis of a similar phase diagram where the BLG bands are now closer to the conduction bands of the TMD, corresponding to Fig. 1b and right column of Table I. Figure 6 shows the resulting phase diagram at two different gate voltages. Apart from having different bandgap map in the $R_1, R_2$ plane, the topological characterization indicates that the heterostructure exhibits only trivial topological phases. This result is a consequence of the larger staggered potential results for this regime (see Table I, $\Delta_1$ and $\Delta_2$). This is intuitively understood as a result of the conduction band in the TMD being dominated by the $d_{z^2}$ orbital and weaker spin-orbit effect there.

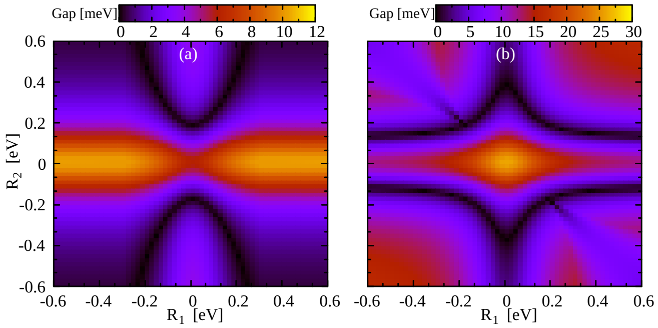


FIG. 6. Map of the bulk spectral gap in BLG-TMD heterostructure as function of $R_1$ and $R_2$ for (a) $V = 0$, and (b) $V = 10$ meV corresponding to effective parameters in the right column of Table I and Fig. 1b. All gapped regions are found to be topologically trivial, characterized by index $Z_2 = +1$, as a consequence of the dominant staggered potential and weaker proximity spin-orbit coupling in this regime.

## V. SYMMETRIC HETEROSTRUCTURE: GRAPHENE-TMD-GRAPHENE

Here, we report results for the structure where the layer order is changed to a symmetric arrangement of graphene-TMD-graphene (G-T-G). The new heterostructure possesses different symmetries and as a result different properties. The tight-binding model is similarly built using the Hamiltonians described in previous sections. The couplings between the TMD and *both* single graphene layers is the same in this case, with both layers set at $R_z = \pm 3.66$ Å, on both sides of the TMD. As a result, the real space lattice structure preserves mirror symmetry around the TMD layer. As before, due to the large separation, the direct coupling between graphene layers is assumed negligible.

### A. Band structure

The band structure along $\Gamma K M \Gamma$ is shown in Fig. 7. Dirac points from both graphene layers at the $K$ valley show linear dispersion ($K'$ valley is similar, with reversed spin states due to TRS). At low-energy, however, we notice two different Dirac bands with qualitatively different structure, where two sets of bands cross away from the $K$ point without mixing. This is due to the mirror symmetry in the $z$-direction that this heterostructure preserves. As such, the eigenvectors of these states can be shown to have parity under layer-inversion, which interchanges graphene layer 1 spinors with graphene layer 2 spinors. Gray bands shown in Fig. 7 are antisymmetric under this inversion, $\langle \psi | I_x | \psi \rangle = -1$, while colored bands are symmetric, $\langle \psi | I_x | \psi \rangle = 1$. The gray color in the antisymmetric bands indicates zero $s_z$-spin, whereas red (blue) show spin up (down) states.

### B. Effective Hamiltonian

The set of orthogonal bands with definite layer inversion parity are easily modeled by an effective Hamiltonian for each symmetry set. Examining spin and staggered expectation value at the $K$ valley shows that the antisymmetric bands have indeed zero $s_z$-spin, whereas colored bands are nearly fully spin-polarized. Gray bands in Fig. 7 are gapless and parabolic due to the existence of only Rashba SOC that changes its Dirac linearity slightly. The other four bands show however more complicated behavior. Along with Rashba SOC, they show intrinsic and diagonal SO terms ($S$ and $\lambda$, respectively), as well as staggered effect ($\Delta$) due to the proximity to a TMDs substrate. This block diagonal effective Hamiltonian is capable of describing well the low energy structure.

### C. Breaking mirror symmetry along z-axis effect

Breaking $z$-axis symmetry can be achieved in two simple ways, as discussed in the main text. One method is by sliding one of the graphene layers horizontally, while a second method is to apply a gate voltage difference across the heterostructure. Both approaches break mirror (layer inversion) symmetry, allowing for level mixing–especially near level crossings. As a result, both blocks in the effective Hamiltonian hybridize and open several gaps in the spectrum. Figure 8 shows band structures of G-T-G in three cases where mirror symmetry is broken in different ways. Interestingly, breaking mirror symmetry by either a small gate voltage across layers or by sliding the layers produces similar gaps and mixings.

Fitting such broken mirror symmetry systems to an effective Hamiltonian requires introducing new momentum-dependent terms that couple the layers, with the form $\frac{a}{2}\left[\lambda^A\left(\sigma_0+\sigma_z\right)+\lambda^B\left(\sigma_0-\sigma_z\right)\right] \times (k_x s_y - k_y s_x)$, with constant parameters $\lambda^{(A/B)}$. Similar terms have been used in Ref. 15 and 16 to mix spin states in single-layer graphene. It is clear, however, that the various gaps in the structure are local in momentum space and do not result in full insulating behavior.

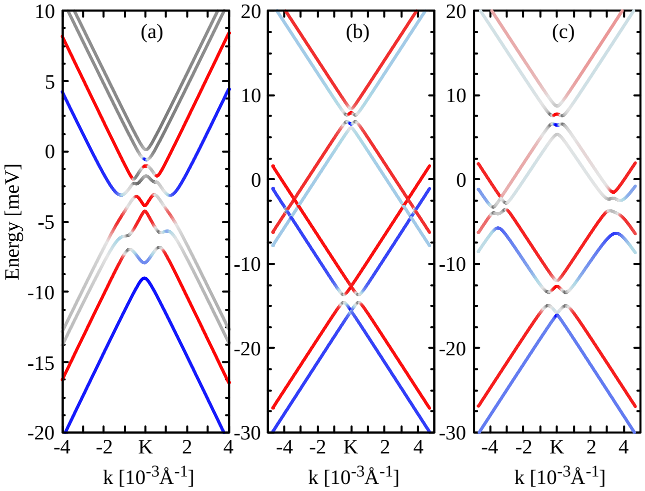


FIG. 8. Bands near the $K$ valley around the Fermi level, shown with different broken mirror cases. (a) Structure produced by spatial displacement of one layer. (b) Bands in the presence of an external voltage. (c) Structure for combined symmetry breaking as in (a) *and* (b). Red (blue) color indicates spin up (down) state texture of bands.

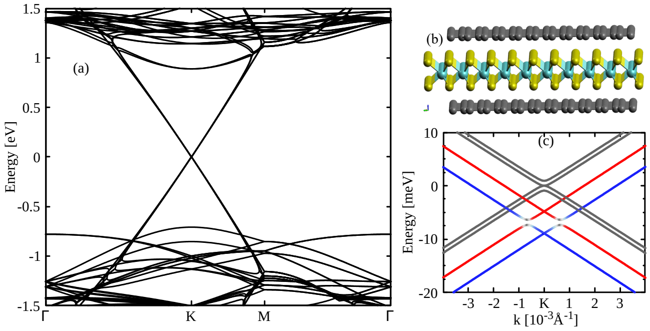


FIG. 7. (a) Γ-$K$-$M$-Γ band structure of coupled graphene-TMD-graphene obtained from tight-binding calculations. (b) Side view of atomic arrangement of TMD and graphene supercell. (c) Magnification for bands at $K$ valley near the Fermi level ($E_F = 0$). Red (blue) lines indicate $s_z$ spin up (down) projection of each band. Gray bands show zero spin.


[1] G.-B. Liu, W.-Y. Shan, Y. Yao, W. Yao, and D. Xiao, Phys. Rev. B **88**, 085433 (2013).

[2] A. H. Castro Neto, F. Guinea, N. M. R. Peres, K. S. Novoselov, and A. K. Geim, Rev. Mod. Phys. **81**, 109 (2009).

[3] J.-W. Jiang and H. S. Park, App. Phys. Lett. **105**, 033108 (2014).

[4] D. Pierucci, H. Henck, J. Avila, A. Balan, C. H. Naylor, G. Patriarche, Y. J. Dappe, M. G. Silly, F. Sirotti, A. T. C. Johnson, M. C. Asensio, and A. Ouerghi, Nano Lett. **16**, 4054 (2016).

[5] A. M. Alsharari, M. M. Asmar, and S. E. Ulloa, Phys. Rev. B **94**, 241106 (2016).

[6] M. Gmitra and J. Fabian, Phys. Rev. Lett. **119**, 146401 (2017).

[7] Z. Wang, D.-K. Ki, H. Chen, H. Berger, A. H. MacDonald, and A. F. Morpurgo, Nat. Commun. **6**, 8339 (2015).

[8] S. Singh and A. H. Romero, unpublished (2018).

[9] J. Jung and A. H. MacDonald, Phys. Rev. B **89**, 035405 (2014).

[10] C. L. Kane and E. J. Mele, Phys. Rev. Lett. **95**, 226801 (2005).
[11] D. Xiao, M.-C. Chang, and Q. Niu, Rev. Mod. Phys. **82**, 1959 (2010).
[12] E. Prodan, Phys. Rev. B **83**, 235115 (2011).
[13] B. Leung and E. Prodan, Phys. Rev. B **85**, 205136 (2012).
[14] F. Geissler, J. C. Budich, and B. Trauzettel, New Journal of Physics **15**, 085030 (2013).
[15] M. Gmitra, D. Kochan, P. Högl, and J. Fabian, Phys. Rev. B **93**, 155104 (2016).
[16] M. Gmitra and J. Fabian, Phys. Rev. B **92**, 155403 (2015).
